# Supplementary material for: Phase Diffusion and Lamb-Shift-Like Spectrum Shift in Classical Oscillators
Source: arXiv:0908.2214 source file (2010-06-24)
Supplement: Supplementary file 1 [file phase-diffusion-PRL-supplemental.pdf]

# Supplemental Material: Complete Calculation of $f(x, \tau)$ and $R_v(\tau)$

Xiaofeng Li, Wenjiang Zhu, and Donhee Ham
School of Engineering and Applied Sciences, Harvard University

June 23, 2010

We here present the complete calculation of $f(x, \tau)$ and $R_v(\tau)$ to any order of accuracy, so as to fill in the details of their calculation that appear in the main manuscript.

## 1 Complete Calculation of $f(x, \tau)$

Since the Feynman-Kac equation:

$$\frac{\partial f}{\partial \tau} = (H_0 + H')f, \tag{1a}$$

$$H_0 = \omega_0 \frac{\partial}{\partial x} + D\frac{\partial^2}{\partial x^2}, \tag{1b}$$

$$H' = D\cos 2x \frac{\partial^2}{\partial x^2}, \tag{1c}$$

has the same form as the Schrödinger equation, we solve it by applying the standard perturbation theory of quantum mechanics, as found in [1]. The $H'$ term acts as a perturbation. When $D \ll \omega_0$, $H'$ becomes negligible compared to $H_0$, and the solution of the nonlinear Langevin equation would converge to the simplified model. Since $H \equiv H_0 + H'$ is not Hermitian, a certain part of the calculation will require a special care, as seen later in Subsec. 1.2, but the general structure of calculation is the same as in quantum mechanics.

Let $\epsilon_n$ and $g_n(x)$ be the $n$-th eigenvalue and eigenstate of (1). They satisfy the following time-independent equation:

$$(H_0 + H')g_n(x) = \epsilon_n g_n(x), \tag{2}$$

Here the quantization with $n = \pm 1, \pm 2, \pm 3, ...$ arises due to the periodic boundary condition $g_n(0) = g_n(2\pi)$. Note that $g_n^*(x)$, the complex conjugate of $g_n(x)$, is also an eigenstate with eigenvalue $\epsilon_n^*$, since $H_0 + H'$ is a real operator. We therefore denote $g_n^*$ and $\epsilon_n^*$ as $g_{-n}$ and $\epsilon_{-n}$. This is why the index $n$ runs over both positive and negative integers. Since $g_n(x)$ evolves with $\tau$ as $e^{\epsilon_n \tau} g_n$, $f(x, \tau)$ can be expressed as a linear combination of the time-evolving eigenstates:

$$f(x, \tau) = \sum_n c_n e^{\epsilon_n \tau} g_n(x), \tag{3}$$

where the coefficients $c_n$'s are set by the initial condition, $f(x, 0) = e^{ix}$. Our task is first to calculate the eigenvalues $\epsilon_n$'s and the eigenstates $g_n(x)$'s using the perturbation technique borrowed from quantum mechanics, and then to determine the coefficients $c_n$'s using the initial condition.

### 1.1 Calculation of $\epsilon_n$ and $g_n(x)$ via Perturbation Technique

To solve the eigenvalue problem of (2) using perturbation method, we introduce a parameter $\lambda$ ($0 \leq \lambda \leq 1$) that can turn the perturbation term, $H'$, "on" ($\lambda = 1$) or "off" ($\lambda = 0$):

$$(H_0 + \lambda H')g_n = \epsilon_n g_n, \tag{4}$$

We may expand $g_n$ and $\epsilon_n$ in power series of $\lambda$,

$$g_n = g_n^{(0)} + \lambda g_n^{(1)} + \lambda^2 g_n^{(2)} + \cdots, \tag{5a}$$
$$\epsilon_n = \epsilon_n^{(0)} + \lambda \epsilon_n^{(1)} + \lambda^2 \epsilon_n^{(2)} + \cdots, \tag{5b}$$

where the superscripts indicate the order of perturbation corrections. By inserting these expressions into (4), we have

$$(H_0 + \lambda H')(g_n^{(0)} + \lambda g_n^{(1)} + \lambda^2 g_n^{(2)} \cdots) = (\epsilon_n^{(0)} + \lambda \epsilon_n^{(1)} + \lambda^2 \epsilon_n^{(2)} \cdots)(g_n^{(0)} + \lambda g_n^{(1)} + \lambda^2 g_n^{(2)} \cdots).$$

Equating the terms with the same order of $\lambda$, we obtain the following set of equations

$$H_0 g_n^{(0)} = \epsilon_n^{(0)} g_n^{(0)}, \tag{6a}$$
$$H_0 g_n^{(k)} + H' g_n^{(k-1)} = \sum_{j=0}^{k} \epsilon_n^{(j)} g_n^{(k-j)} \qquad (k = 1, 2, 3, \cdots). \tag{6b}$$

By solving the unperturbed equation (6a) in connection with the periodic boundary condition, we obtain the unperturbed eigenvalues $\epsilon_n^{(0)}$'s and the unperturbed eigenstates $g_n^{(0)}(x)$'s (the 0th-order solution):

$$g_n^{(0)}(x) = e^{inx} \text{ and } \epsilon_n^{(0)} = in\omega_0 - n^2 D. \tag{7}$$

Although $H_0$ is not Hermitian, $\{g_n^{(0)}\}$ *happens* to form an orthogonal set (as we will discuss shortly in Subsec. 1.2, only the unperturbed eigenstates, $g_n^{(0)}$'s, are orthogonal, and orthogonality will *not* hold for $g_n$'s that include higher-order correction terms):

$$\frac{1}{2\pi} \int_0^{2\pi} g_n^{(0)*}(x) \cdot g_m^{(0)}(x) = \delta_{nm}. \tag{8}$$

The $k$th-order correction term in the $n$-th eigenstate $g_n$ can be expanded using $\{g_n^{(0)}\}$ as basis:

$$g_n^{(k)}(x) = \sum_m a_{n,m}^{(k)} g_m^{(0)}(x). \tag{9}$$

After plugging (9) into (6b), we multiply both sides of (6b) by $(g_m^{(0)})^*$ and integrate them from 0 to $2\pi$ (to exploit the orthogonality of $\{g_n^{(0)}\}$) to attain

$$\epsilon_n^{(k)} = \sum_m a_{n,m}^{(k-1)} H'_{nm} - \sum_{j=1}^{k-1} \epsilon_n^{(j)} a_{n,n}^{(k-j)}; \tag{10a}$$

$$a_{n,m}^{(k)} = \begin{cases} \dfrac{1}{\epsilon_n^{(0)} - \epsilon_m^{(0)}} \left[ \sum_l a_{n,l}^{(k-1)} H'_{ml} - \sum_{j=1}^{k-1} \epsilon_n^{(j)} a_{n,m}^{(k-j)} \right] & (m \neq n), \\ -\dfrac{1}{2} \left[ \sum_{j=1}^{k-1} a_{n,n}^{(j)} a_{n,n}^{(k-j)} + \sum_{l \neq n} \sum_{j=1}^{k-1} (a_{n,l}^{(j)})^* a_{n,l}^{(k-j)} \right] & (m = n). \end{cases} \tag{10b}$$

where $H'_{mn}$ is the matrix element of $H'$, with the unperturbed eigenstates $g_n^{(0)}$'s as basis:

$$H'_{mn} \equiv \frac{1}{2\pi} \int_0^{2\pi} (g_m^{(0)})^* H' g_n^{(0)} dx = -\frac{n^2 D}{2} \delta_{m,n\pm 2}. \tag{11}$$

In determining $a_{n,n}^{(k)}$ (*i.e.*, the $m = n$ case), we have used the normalization condition $|g_n|^2 = |g_n^{(0)} + \lambda g_n^{(1)} + \cdots + \lambda^k g_n^{(k)} + \cdots|^2 = 1$ and matched the terms up to the order of $\lambda^k$. Using the recursive formulae (10), the $k$th order corrections $\epsilon_n^{(k)}$ and $a_{n,m}^{(k)}$ can be computed from the lower-order ones $\epsilon_n^{(j)}$ and $a_{n,m}^{(j)}$ $(0 \leq j \leq k-1)$. This concludes the calculation of the eigenvalues $\epsilon_n$'s and the eigenstates $g_n(x)$'s to any order of accuracy.

## 1.2 Determination of $c_n$

The coefficients $c_n$'s in (3) are to be determined from the initial condition

$$f(x,0) = e^{ix} = \sum_n c_n g_n(x). \tag{12}$$

where the eigenstates $g_n(x)$'s are known to any order of accuracy from the procedure of Subsec. 1.1. The above equation is an expansion of $e^{ix}$ in terms of the eigenstates $g_n(x)$'s. A usual method to calculate the coefficients $c_n$'s in equations like (12) is to utilize the orthogonality among the eigenstates. Such convenience, however, is not apparently available in our case, as $\{g_n\}$ is not an orthogonal set due to the non-Hermiticity of $H = H_0 + H'$:

$$\int_0^{2\pi} g_m^*(x) \cdot g_n(x) dx \neq 0 \quad \text{for} \quad m \neq n.$$

(By contrast, orthogonality holds for the unperturbed eigenstates, $g_n^{(0)}$'s, as seen earlier). But the calculation of $c_n$ can be still easily done, if we exploit the eigenstates of the adjoint operator $H^\dagger = (H_0 + H')^\dagger$:

$$H^\dagger = -\omega_0 \frac{\partial}{\partial x} + 2D \frac{\partial^2}{\partial x^2} \cos^2 x. \tag{13}$$

Let $h_n(x)$ and $\mu_n$ be the $n$-th eigenstate and eigenvalue of $H^\dagger$. Then we have $H^\dagger h_n(x) = \mu_n h_n(x)$, which is essentially the Fokker-Planck equation in its time-independent form:

$$-\omega_0 \frac{\partial h_n}{\partial x} + 2D \frac{\partial^2}{\partial x^2} \left(\cos^2 x \cdot h_n\right) = \mu_n h_n. \tag{14}$$

By solving this equation using the same perturbation technique of Subsec. 1.1, $h_n(x)$ and $\mu_n$ can be calculated to any order of accuracy.

For further development, we define the inner product of two functions, $\xi(x)$ and $\eta(x)$, as

$$(\xi, \eta) \equiv \frac{1}{2\pi} \int_0^{2\pi} \xi^*(x) \eta(x) dx. \tag{15}$$

If $\xi(x)$ and $\eta(x)$ are periodic in $2\pi$, we have

$$(\xi, H\eta) = (H^\dagger \xi, \eta), \tag{16}$$

which can be verified from the following identity obtained by integration by parts, together with the periodicity of $\xi(x)$ and $\eta(x)$:

$$\int_0^{2\pi} \xi^* \left(\omega_0 \frac{\partial \eta}{\partial x} + 2D \cos^2 x \frac{\partial^2 \eta}{\partial x^2}\right) dx = \int_0^{2\pi} \left(-\omega_0 \frac{\partial \xi}{\partial x} + 2D \frac{\partial^2}{\partial x^2} \left(\cos^2 x \cdot \xi\right)\right)^* \eta dx.$$

Now let us see how the eigenstates $h_n$'s of $H^\dagger$ come to rescue in calculation of $c_n$. To begin with, if $\epsilon_n$ is an eigenvalue of $H$, $\epsilon_n^*$ must be an eigenvalue of $H^\dagger$. This may be easily seen in the matrix representation. Due to (16), the matrix for $H^\dagger$ is the conjugate transpose of that of $H$, in any basis consisting of functions periodic in $2\pi$. It then follows from the well-known property of complex conjugate matrices that if $\epsilon_n$ is an eigenvalue of $H$, $\epsilon_n^*$ must be an eigenvalue of $H^\dagger$. Thus we use the same $n$ for $h_n$ and $g_n$ when their corresponding eigenvalues are complex conjugates: $\mu_n = \epsilon_n^*$. Now according to (16), we have

$$\begin{aligned} & (h_n, Hg_m) = (h_n, \epsilon_m g_m) = \epsilon_m (h_n, g_m), \\ = \quad & (H^\dagger h_n, g_m) = (\mu_n h_n, g_m) = \mu_n^* (h_n, g_m) = \epsilon_n (h_n, g_m), \end{aligned}$$

where we have used $\mu_n = \epsilon_n^*$ in the second line. Thus, for $m \neq n$, $(h_n, g_m) = 0$, as there is no degeneracy in $\epsilon_n$'s. Therefore, with proper normalization, $\{h_n(x)\}$ form an orthonormal dual basis of $\{g_n(x)\}$:

$$(h_n, g_m) = \frac{1}{2\pi} \int_0^{2\pi} h_n^*(x) \cdot g_m(x) dx = \delta_{nm}. \tag{17}$$

Applying this orthonormal relation to (12), $c_n$ is determined as

$$c_n = (h_n, e^{ix}) = \frac{1}{2\pi}\int_0^{2\pi} h_n^*(x) e^{ix} dx. \tag{18}$$

In the following subsections, we apply the results of Subsecs. 1.1 and 1.2 to calculate $f(x,\tau)$ explicitly to increasing orders of accuracy.

### 1.3 Calculation of the Unperturbed $f(x,\tau)$

The unperturbed ($H' = 0$) eigenstates and eigenvalues are given by (7). The initial condition $f(x,0) = e^{ix}$ is already an eigenstate, $g_1^{(0)}(x)$, of $H_0$, thus, $f(x,\tau) = e^{\epsilon_1^{(0)}\tau} g_1^{(0)}(x) = e^{-D\tau} e^{i(\omega_0\tau + x)}$ with no other eigenstates excited: $c_1 = 1$. This corresponds to the solution of the simplified model.

### 1.4 Calculation of $f(x,\tau)$ to the Lowest Order

Plugging $k = 1$, $a_{n,m}^{(0)} = \delta_{nm}$, and $H'_{nm}$ of (11) into (10) yields

$$\epsilon_n^{(1)} = H'_{nn} = 0; \tag{19a}$$

$$a_{n,m}^{(1)} = \begin{cases} \dfrac{H'_{mn}}{\epsilon_n^{(0)} - \epsilon_m^{(0)}} = \dfrac{n^2 D/4}{\pm i\omega_0 - 2(\pm n + 1)D} & (m = n \pm 2), \\ 0 & (\text{otherwise}). \end{cases} \tag{19b}$$

Given (19b), $g_n$, to the 1st order, is

$$\begin{aligned} g_n &= g_n^{(0)} + a_{n,n+2}^{(1)} g_{n+2}^{(0)} + a_{n,n-2}^{(1)} g_{n-2}^{(0)} \\ &= e^{inx} + \frac{n^2 D/4}{i\omega_0 - 2(n+1)D} e^{i(n+2)x} - \frac{n^2 D/4}{i\omega_0 - 2(n-1)D} e^{i(n-2)x} \end{aligned} \tag{20}$$

By contrast, the 1st order correction to $\epsilon_n$ vanishes as $H'_{nn} = 0$. Therefore, it is necessary to go to the 2nd order to obtained the lowest-order correction to $\epsilon_n$. Using $k = 2$ and (19) in the recursive formula (10a), we have:

$$\epsilon_n^{(2)} = \sum_{m \neq n} \frac{H'_{mn} H'_{nm}}{\epsilon_n^{(0)} - \epsilon_m^{(0)}} = \frac{n^2(n+2)^2 D^2/4}{-i2\omega_0 + 4(n+1)D} + \frac{n^2(n-2)^2 D^2/4}{i2\omega_0 - 4(n-1)D}, \tag{21}$$

This concludes the calculation for the lowest-order eigenvalues and eigenstates.

To determine $c_n$ according to the strategy of Subsec. 1.2, we first calculate the eigenstates $h_n$ of $H^\dagger$ to the 1st order by solving (14) using the same perturbation technique as used in Subsec. 1.1:

$$h_n = e^{inx} - \frac{(n+2)^2 D/4}{i\omega_0 + 2(n+1)D} e^{i(n+2)x} + \frac{(n-2)^2 D/4}{i\omega_0 + 2(n-1)D} e^{i(n-2)x}. \tag{22}$$

Note that $(h_m, g_n) = \delta_{mn}$ to the 1st order of $D/\omega_0$, which meets the general orthogonality property (17). We use $h_n$ in (18) to compute $c_n$:

$$\begin{aligned} c_1 &= \frac{1}{2\pi}\int_0^{2\pi} h_1^*(x) e^{ix} dx = 1, \\ c_{-1} &= \frac{1}{2\pi}\int_0^{2\pi} h_{-1}^*(x) e^{ix} dx = \frac{D}{i4\omega_0}, \\ c_3 &= \frac{1}{2\pi}\int_0^{2\pi} h_3^*(x) e^{ix} dx = \frac{D}{4(-i\omega_0 + 4D)}. \end{aligned}$$

All other coefficients vanish up to the 1st order. Note that $|c_1| = 1$ is larger than $|c_{-1}|$ and $|c_3|$, because $f(x, 0) = g_1^{(0)}(x)$ is still close to $g_1(x)$.

With $g_n$, $\epsilon_n$, and $c_n$ computed so far to the lowest order, we can readily write $f(x, \tau)$ to the same order as

$$f(x,\tau) = e^{\epsilon_1 \tau} g_1(x) + c_{-1} e^{\epsilon_1^* \tau} g_1^*(x) + c_3 e^{\epsilon_3 \tau} g_3(x).$$

where we have used $g_{-1} = g_1^*$ and $\epsilon_{-1} = \epsilon_1^*$. As the decay rate $\sim n^2 D = 9D$ of $e^{\epsilon_3 \tau}$ is far larger than the decay rate $\sim n^2 D = D$ of $e^{\epsilon_1 \tau}$ and $e^{\epsilon_1^* \tau}$, the last term can be dropped to yield

$$f(x,\tau) \approx e^{\epsilon_1 \tau} g_1(x) + \frac{D}{i4\omega_0} e^{\epsilon_1^* \tau} g_1^*(x). \tag{23}$$

Here,

$$g_1 = g_1^{(0)} + a_{1,-1}^{(1)} g_{-1}^{(0)} + a_{1,3}^{(1)} g_3^{(0)} = e^{ix} - \frac{D}{i4\omega_0} e^{-ix} + \frac{D/4}{i\omega_0 - 4D} e^{i3x}, \tag{24a}$$

$$\epsilon_1 = \epsilon_1^{(0)} + \epsilon_1^{(2)} = i(\omega_0 + \beta) - (D - \alpha), \tag{24b}$$

where $\alpha \equiv \mathrm{Re}[\epsilon_1 - \epsilon_1^{(0)}]$ and $\beta \equiv \mathrm{Im}[\epsilon_1 - \epsilon_1^{(0)}]$ (in the current, lowest-order calculation, $\alpha = \mathrm{Re}[\epsilon_1^{(2)}]$ and $\beta = \mathrm{Im}[\epsilon_1^{(2)}]$) are

$$\alpha = (9/2)[D^2/(16D^2 + \omega_0^2)]D; \tag{25a}$$

$$\beta = (D/8)[9D\omega_0/(16D^2 + \omega_0^2) - D/\omega_0], \tag{25b}$$

as given in the main manuscript. The correction of the eigenvalue by $-\alpha$ in the real part and $\beta$ in the imaginary part represents the diffusion rate reduction from $D$ and the oscillation frequency blue shift, which are of physical significance, as detailed in the main manuscript.

### 1.5 Calculation of $f(x, \tau)$ to Higher Orders

We can readily extend the lowest-order calculation of $f(x, \tau)$ to any higher order of accuracy in a recursive fashion using the formulae (10). In the lowest-order calculation of the foregoing subsection, only 3 eigenstates, $g_1$, $g_{-1}$, and $g_3$, were excited (with $g_3$ decaying very fast). In higher order, a larger number of eigenstates are excited. However, we can still write $f(x, \tau)$ as

$$f(x,\tau) \approx c_1 e^{\epsilon_1 \tau} g_1(x) + c_{-1} e^{\epsilon_1^* \tau} g_1^*(x), \tag{26}$$

because other terms decay much faster (decay rate $\sim n^2 D$) than $e^{\epsilon_1 \tau}$ and $e^{\epsilon_1^* \tau}$ (decay rate $\sim D$). Secondarily, $|c_1|$ is larger than other $|c_n|$'s due to the initial condition. Thus, we can focus on $\epsilon_1$ and $g_1$ even in higher-order calculations. The difference of (26) from (23) is that the reduction $\alpha$ of the effective phase diffusion rate and the oscillation frequency shift $\beta$ (as well as the coefficients $c_1$ and $c_{-1}$) are made more accurate through the higher order corrections. The computation of $\alpha = \mathrm{Re}[\epsilon_1 - \epsilon_1^{(0)}]$ and $\beta = \mathrm{Im}[\epsilon_1 - \epsilon_1^{(0)}]$ for $D/\omega_0 = 1$, $1/2$, and $1/4$ up to the order of $k = 100$ is shown in Fig. S1, which demonstrates the convergence of the higher order corrections.

## 2 Complete Calculation of $R(\tau)$

To compute the autocorrelation of Eq. (4) of the main manuscript, we should perform the integrations in Eq. (5) of the main manuscript. Since $f(x, \tau)$ has been calculated in Sec. 1, the remaining job is to find the stationary probability density $p(x)$ of $\psi = x$, which appears in Eq. (5) of the main manuscript. The transient probability density $p(x, t)$ satisfies the following Fokker-Planck equation

$$\frac{\partial p}{\partial t} = -\omega_0 \frac{\partial p}{\partial x} + 2D \frac{\partial^2}{\partial x^2}(p \cos^2 x),$$

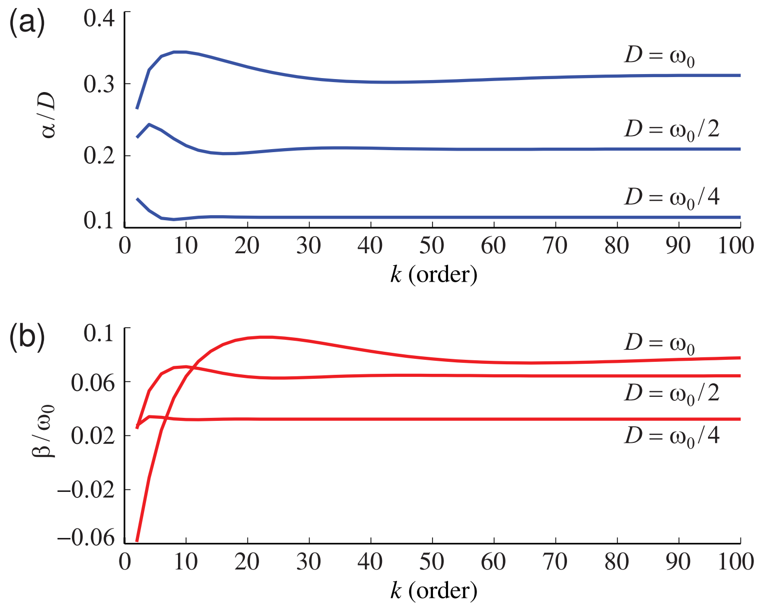


Figure S1: $\alpha$ and $\beta$ obtained by calculations up to the 100th order.

which is commensurate with the nonlinear Langevin equation for $\psi$ given in Eq. (3) of the main manuscript. If we set $\partial p/\partial t = 0$, the equation above reduces to

$$\frac{2D}{\omega_0}\frac{\partial^2}{\partial x^2}(p\cos^2 x) - \frac{\partial p}{\partial x} = 0, \tag{27}$$

which the stationary probability density $p(x)$ must satisfy. $p(x)$ should also satisfy the periodic boundary condition $p(0) = p(2\pi)$. When $D \ll \omega_0$, the above equation becomes $\partial p/\partial x = 0$, and $p$ assumes a uniform distribution. The exact $p(x)$ can be obtained in closed form, by solving (27) with the periodic boundary condition and the normalization condition $\int_0^{2\pi} p dx = 1$:

$$p(x) = \begin{cases} \dfrac{\omega_0}{4\pi D}(1+\tan^2 x)e^{(\omega_0/2D)\tan x}\displaystyle\int_{-\infty}^{-\tan x}\frac{e^{(\omega_0/2D)y}}{1+y^2}dy \\ \dfrac{1}{2\pi} & (x = \pi/2,\ 3\pi/2). \end{cases} \tag{28}$$

## 2.1 Calculation of $R_v(\tau)$ to the Lowest Order

Let us first assume a uniform stationary probability density for $x$, that is, $p(x) = 1/2\pi$, which is accurate for $D \ll \omega_0$. Using this uniform $p(x)$ and the lowest-order $f(x,\tau)$ of (23) in Eqs. (4) and (5) of the main manuscript, and keeping the coefficients to the 1st order of $D/\omega_0$, we obtain

$$\left\langle e^{i[\psi(t+\tau)-\psi(t)]}\right\rangle = \frac{1}{2\pi}\int_0^{2\pi} f(x,\tau)e^{-ix}dx = e^{\epsilon_1\tau} - \frac{D^2}{16\omega_0^2}e^{\epsilon_1^*\tau} \approx e^{\epsilon_1\tau}, \tag{29}$$

$$\left\langle e^{i[\psi(t+\tau)+\psi(t)]}\right\rangle = \frac{1}{2\pi}\int_0^{2\pi} f(x,\tau)e^{ix}dx = -\frac{D}{i4\omega_0}e^{\epsilon_1\tau} + \frac{D}{i4\omega_0}e^{\epsilon_1^*\tau}, \tag{30}$$

$$R_v(\tau) = \frac{v_0^2}{2}e^{-(D-\alpha)|\tau|}\left[\cos(\omega_0+\beta)\tau - \frac{D}{2\omega_0}\sin(\omega_0+\beta)|\tau|\right], \tag{31}$$

where $\alpha$ and $\beta$ are given by (25).

Let us see how the exact $p(x)$ alters $R_v(\tau)$. If we use the general $f(x,\tau)$ expression of (3) in Eqs. (4) and (5) of the main manuscript, we obtain

$$R_v(\tau) = \frac{v_0^2}{2} \sum_n \mathrm{Re} \left[ c_n e^{\epsilon_n \tau} \int_0^{2\pi} g_n(x)(e^{-ix} + e^{ix}) p(x) dx \right]. \tag{32}$$

Since the eigenvalues $\epsilon_n$ are determined in the process of solving for $f(x,\tau)$, which is independent of using $p(x)$ in the integration above, each term in (32) has the same decay rate and frequency shift as before when the approximate, uniform $p(x)$ was used. The only difference is the slightly modified coefficients given by $c_n \int_0^{2\pi} g_n(x)(e^{-ix} + e^{ix}) p(x) dx$. Therefore, the essence of our results, especially the physically important decay rate reduction and frequency shift, remains unaltered, whether or not we use the exact $p(x)$. For example, when $D = \omega_0/4$, the exact $p(x)$ and the lowest-order $f(x,\tau)$ of (23) give

$$R_v(\tau) = \frac{v_0^2}{2} e^{-(D-\alpha)|\tau|} [0.91 \cos(\omega_0 + \beta)\tau + 0.08 \sin(\omega_0 + \beta)|\tau|], \tag{33}$$

while (31) obtained for the approximate, uniform $p(x)$ and the lowest-order $f(x,\tau)$ of (23) becomes

$$R_v(\tau) = \frac{v_0^2}{2} e^{-(D-\alpha)|\tau|} [\cos(\omega_0 + \beta)\tau - 0.125 \sin(\omega_0 + \beta)|\tau|]. \tag{34}$$

We can always use the exact non-uniform $p(x)$ to attain more accurate result, but the essence of the result is not altered. As can be seen in both $R_v(\tau)$'s above, the coefficients are slightly modified (although the second term changes the sign, its effect is negligible as it is far weaker than the first term), but the functional form remains the same with the same $\alpha$ and $\beta$ of (25).

## 2.2 Calculation of $R_v(\tau)$ to Higher Orders

Since $f(x,\tau)$ can be calculated up to any order of accuracy in the form of (26) and the exact $p(x)$ is given in (28), we can obtain $R_v(\tau)$ to any order of accuracy. The functional form of (31) with two dominant terms will remain the same, while the coefficients of the two terms will differ, and $\alpha$ and $\beta$ are made more accurate due to the higher-order corrections.

# References


[1] J. J. Sakurai, *Modern Quantum Mechanics* (Revised Edition), Addison-Wesley, 1993.
